# Supplementary material for: Unifying pendulum-like dynamical regimes via complex time
Source: arXiv:2504.16816 source file (2026-11-03)
Supplement: Supplementary file 1 [file supplemental_material.pdf]

# Supplemental Material

## Simple and exact nonlinear pendulum motion for all possible initial conditions

Teepanis Chachiyo [teepanisc@nu.ac.th](mailto:teepanisc@nu.ac.th) Department of Physics, Faculty of Science, Naresuan University, Phitsanulok 65000, Thailand.

Available at a GitHub repository: <https://github.com/teepanis/nonlinear-pendulum>

This python notebook tests that proposed formulae as compared to the exact numerical solution.

```
In [1]: import numpy as np
import scipy as sp
import matplotlib.pyplot as plt

g = 9.8
L = g/4/np.pi**2
omegac = 2*np.sqrt(g/L)

def theta_exact(omegaM, t):

    E = (1/2*omegaM**2)*L/g
    k = np.sqrt(L/g)*omegaM/2
    theta = np.zeros(len(t))

    for i in range(len(t)):

        if omegaM < omeagac:
            [sn, cn, dn, ph] = sp.special.ellipj(np.sqrt(g/L)*t[i], k**2)
            theta[i] = 2*np.arcsin(k*sn)
        else:
            [sn, cn, dn, ph] = sp.special.ellipj(np.sqrt(g/L)*t[i]*np.sqrt(E/2),
                                                np.sqrt(2/E)**2)
            theta[i] = 2*ph

    return theta

def K_exact(k):
    # scipy defines K differently, so that we need to pass k**2 instead of k
    return sp.special.ellipk(k**2)

def K_thiswork(k):
    n = (np.log(4) - np.log(np.pi))/(np.pi/2 - np.log(4))
    b = np.exp(n*np.pi/2) - 4**n
    return 1/n*np.log( (4/np.sqrt(1-k**2))**n + b)

#mode='exact'
mode='accurate'

def K(k):
    if mode=='exact': return K_exact(k)
    if mode=='accurate': return K_thiswork(k)

##
## the Chiang Khrua solutions (CKS)
##
def theta_CKS(omegaM, t, delta=0):

    theta = np.zeros(len(t))

    N = 20
    # swinging motion
    if omegaM < omeagac:

        # compute period
        k = np.sqrt(L/g)*omegaM/2
        T = 4*np.sqrt(L/g)*K(k)
```

```

# compute coefficients
a = np.zeros(N)
kappa = K(np.sqrt(1-k**2))/K(k)
for n in range(1,N,2):
    a[n] = 4/n/np.cosh(kappa*n*np.pi/2)

# sum contributions at time t
for i in range(len(t)):
    s = 0
    for n in range(0,N): s = s + a[n]*np.sin(2*n*np.pi/T*t[i] + n*delta)
    theta[i] = s

# stopping motion
elif omegaM == omegac:
    for i in range(len(t)):
        theta[i] = 2*np.arcsin( np.tanh(np.sqrt(g/L)*t[i] + delta) )

# spinning motion
else:
    # compute period
    k = np.sqrt(L/g)*omegaM/2
    T = 2*np.sqrt(L/g)/k*K(1/k)

    # compute coefficients
    b = np.zeros(N)
    kappa = K(np.sqrt(1-1/k**2))/K(1/k)
    for n in range(1,N):
        b[n] = 2/n/np.cosh(n*np.pi*kappa)

    # sum contributions at time t +
    for i in range(len(t)):
        s = 0
        for n in range(0,N): s = s + b[n]*np.sin(2*n*np.pi/T*t[i] + n*delta)
        theta[i] = 2*np.pi/T*t[i] + delta + s

return theta

Tmax = 4
t = np.arange(0, Tmax, 0.01)

plt.plot(t, theta_exact(omegac-0.001,t), 'k.', markevery=10, label='Exact Numerical')
plt.plot(t, theta_exact(omegac,t), 'k.', markevery=10)
plt.plot(t, theta_exact(omegac+0.001,t), 'k.', markevery=10)
plt.plot(t, theta_CKS(omegac-0.001,t), 'b--', label='Swinging:  $\omega_m < \omega_c$ ')
plt.plot(t, theta_CKS(omegac,t), 'g-.', label='Stopping:  $\omega_m = \omega_c$ ')
plt.plot(t, theta_CKS(omegac+0.001,t), 'r-', label='Spinning:  $\omega_m > \omega_c$ ')
plt.ylim(-np.pi, 4*np.pi)
plt.xlim(0, Tmax)
plt.yticks([-np.pi, 0, np.pi, 2*np.pi, 3*np.pi, 4*np.pi],
           ['$-\pi$', '0', '$\pi$', '$2\pi$', '$3\pi$', '$4\pi$'])
plt.xticks([0, 1, 2, 3, 4])
plt.grid()
plt.legend()
plt.xlabel('Time [seconds]')
plt.ylabel('Angular Displacement')
#plt.savefig('fig1.pdf')
plt.show()

```

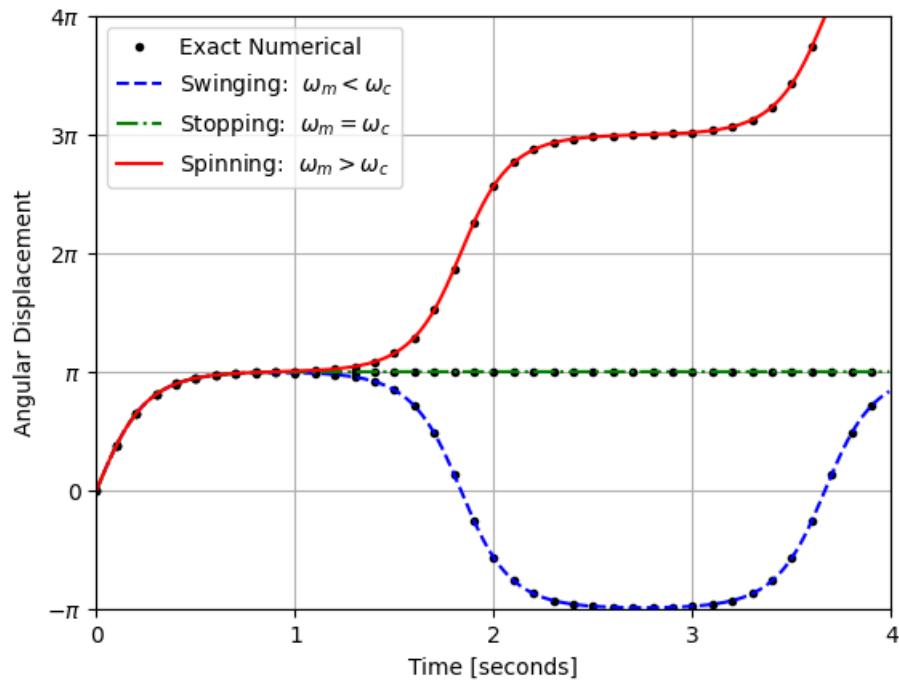

## Exact Solution $K(k)$

```
In [2]: import numpy as np
import scipy
import matplotlib.pyplot as plt

# allocate amplitude theta0 and x
theta0 = np.arange(0, np.pi, .004)
x = np.sin(theta0/2)
N = len(x)

# compute exact K(x)
# Notes: scipy defines the arguments of elliptic function
# differently, so that the x**2 is used instead of just x.
K_exact = scipy.special.ellipk(x**2)

# allocate array for comparisons
K_asym = np.zeros(N)
K_t4 = np.zeros(N)
K_ThisWork = np.zeros(N)
K_lima2008 = np.zeros(N)
K_ganley1985 = np.zeros(N)

for i in range(N):

    # (Lima 2008)
    if x[i] > 0.0:
        a = np.sqrt(1-x[i]**2)
        K_lima2008[i] = np.pi/2*( a**2/(1-a)*np.log(1/a) + 2*x[i]**2/np.pi*np.log(4/a) )
    else:
        K_lima2008[i] = np.pi/2

    K_asym[i] = np.log(4/np.sqrt(1-x[i]**2))
    K_t4[i] = np.pi/2*(1 + 1/4*x[i]**2 + ((1*3)/(2*4))*x[i]**4 )

    # (Ganley 1985)
    alpha = np.sqrt(3)/2*theta0[i]
    if alpha > 0.0: K_ganley1985[i] = np.pi/2*np.sqrt(alpha/np.sin(alpha))
    else: K_ganley1985[i] = 1.0

    n = (np.log(4) - np.log(np.pi))/(np.pi/2 - np.log(4))
    b = np.exp(n*np.pi/2) - 4**n
    K_ThisWork[i] = 1/n*np.log( (4/np.sqrt(1-x[i]**2))**n + b)

plt.plot(x, K_exact*2/np.pi, '.', markevery=20, label='Exact Numerical')
plt.plot(x, K_asym*2/np.pi, '-', label='Asymptotic')
plt.plot(x, K_t4*2/np.pi, '--', label='4th Order Taylor')
plt.plot(x, K_ThisWork*2/np.pi, linewidth=1, label='This Work')
```

```

plt.text(18/180,1.95,'$K(k) \approx \frac{1}{n}$ '
#       '$\ln [ \left(\frac{4}{\sqrt{1-k^2}}\right)^n + b ]$', fontsize=14, \
#       bbox=dict(facecolor='white', alpha=0.9, edgecolor='black', linewidth=0.7))

plt.title('Complete Elliptical Integral of the First Kind')
plt.xlabel('$k$')
plt.ylabel('$K(k) \div \frac{\pi}{2}$')
plt.ylim([.5,3])
plt.xlim([0,1])
plt.legend()
plt.grid()
plt.savefig('fig2.pdf')
plt.show()

```

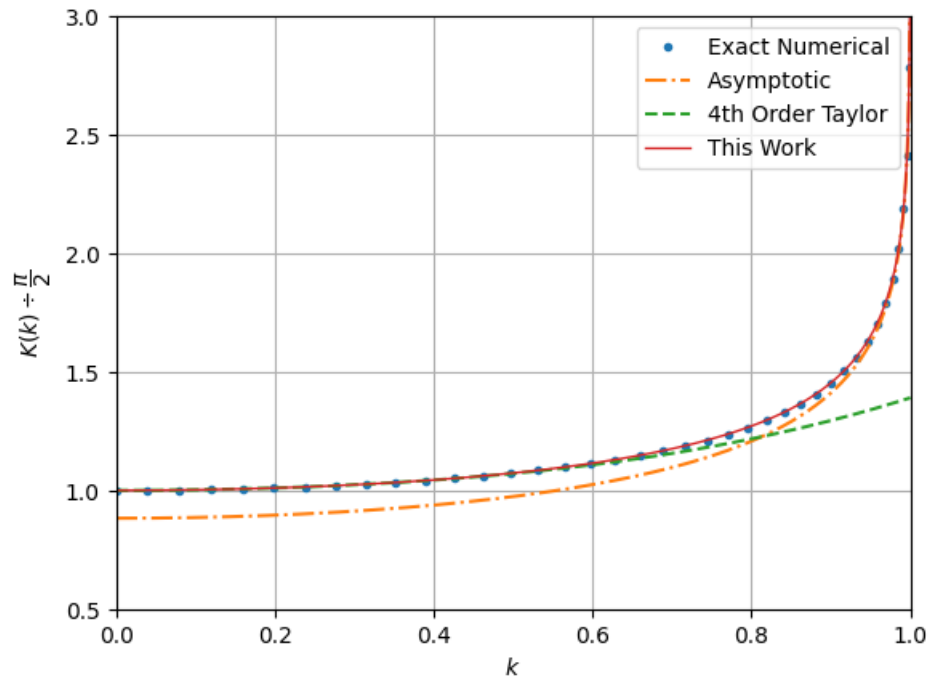

## Comparisons to Existing Analytical Forms

```

In [3]: #
# Error comparison
#

plt.plot(x, np.abs(K_ganley1985-K_exact)*100./K_exact,':', label='Ganley 1985')
plt.plot(x, np.abs(K_lima2008-K_exact)*100./K_exact,'-.', label='Lima 2008')
plt.plot(x, np.abs(K_t4-K_exact)*100./K_exact,'--', label='4th Order Taylor')
plt.plot(x, np.abs(K_ThisWork-K_exact)*100./K_exact, label='This Work')

plt.title('Error compared to the exact K(k)')
plt.xlabel('k')
plt.ylabel('% |Error|')
plt.xlim([0,1])
plt.ylim(0,4)
plt.legend()
plt.grid()
plt.show()
plt.savefig('fig3.pdf')

print('Maximum % |Error|')
print('Lima 2008: %.2f' % ( max(np.abs(K_lima2008-K_exact)*100./K_exact) ) )
print('This Work: %.2f' % ( max(np.abs(K_ThisWork-K_exact)*100./K_exact) ) )

print('\nAverage % |Error|')
print('Lima 2008: %.2f' % ( np.average(np.abs(K_lima2008-K_exact)*100./K_exact) ) )
print('This Work: %.2f' % ( np.average(np.abs(K_ThisWork-K_exact)*100./K_exact) ) )

```

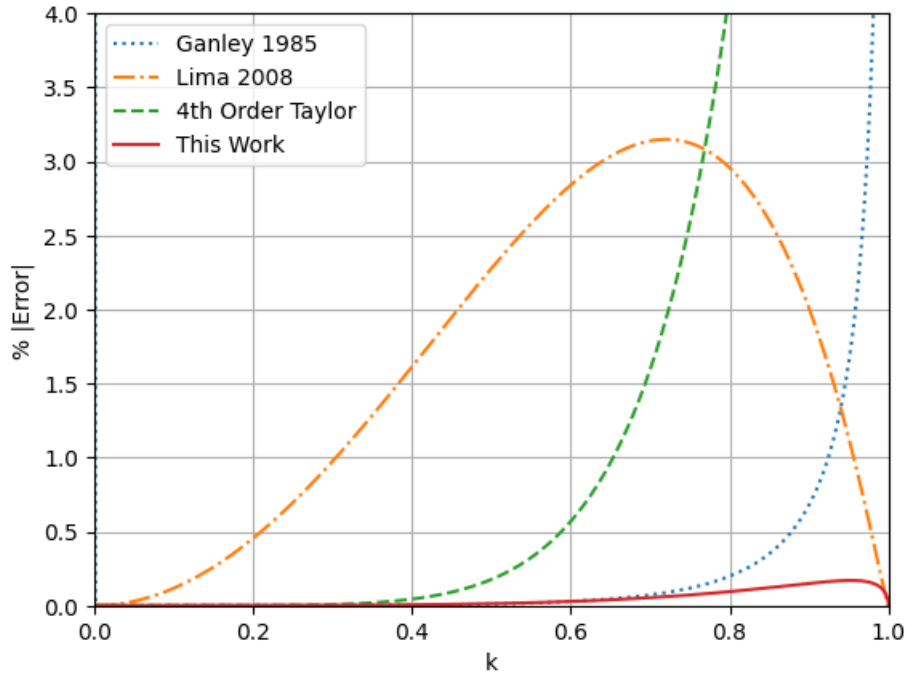

Maximum % |Error|  
Lima 2008: 3.15  
This Work: 0.17

Average % |Error|  
Lima 2008: 1.56  
This Work: 0.06

## Derivation of the Constant $n$ and $b$ in Eq. (8)

Below is a python code that symbolically derivatives of the proposed form, evaluated at  $x = 0$ . The derivatives can then be compared to that of the exact  $K(x)$ . Demanding that they agree upto the 2nd order will ensure that the proposed form approaches the exact limit when the amplitudes is small.

```
In [4]: ## checking taylor expansion of the proposed form
##
import sympy as sym

xx = sym.symbols('x', real=True)
bb = sym.symbols('b', real=True)
nn = sym.symbols('n', real=True)

# the proposed form
K0 = 1/nn*sym.ln((4/sym.sqrt(1-xx**2))*nn + bb)

print('0th Derivative: ', K0.subs(xx,0))
K1 = K0.diff(xx)
print('1st Derivative: ', K1.subs(xx,0))
K2 = K1.diff(xx)
print('2nd Derivative: ', K2.subs(xx,0))
K3 = K2.diff(xx)
print('3rd Derivative: ', K3.subs(xx,0))

0th Derivative: log(4**n + b)/n
1st Derivative: 0
2nd Derivative: 4**n/(4**n + b)
3rd Derivative: 0
```

Taylor series (sometimes called power series) of the exact  $K(x)$  is

$$K(x) = \frac{\pi}{2} \left[ 1 + \left( \frac{1}{2} \right)^2 x^2 + \left( \frac{1 \cdot 3}{2 \cdot 4} \right)^2 x^4 + \left( \frac{1 \cdot 3 \cdot 5}{2 \cdot 4 \cdot 6} \right)^2 x^6 + \dots \right] \quad (\text{S2})$$

Therefore,  $K(0) = \frac{\pi}{2}$  and  $K''(0) = \frac{\pi}{4}$ . From the output of the python code above, it follows that

$$\frac{1}{n} \log(4^n + b) = \frac{\pi}{2} \quad (\text{S3})$$

$$\frac{4^n}{4^n + b} = \frac{\pi}{4} \quad (\text{S4})$$

which lead to

$$n = \frac{\ln 4 - \ln \pi}{\pi/2 - \ln 4} \quad \text{and} \quad b = e^{n\pi/2} - 4^n$$

## Derivation the CKS in Eq. (2)

The equation of motion for a physical pendulum reads

$$\frac{d^2\theta}{dt^2} + \frac{LMg}{I} \sin \theta = 0 \quad (\text{S5})$$

$L$  is the distance from a pivot point to the center of mass.  $I$  is the moment of inertia about the pivot point. For a simple pendulum,  $I = ML^2$ ; so the equation of motion reduces to

$$\frac{d^2\theta}{dt^2} + \frac{g}{L} \sin \theta = 0 \quad (\text{S6})$$

The above form is still inconvenient to work with due to the factor  $\frac{g}{L}$  that would have to tag along throughout the derivations. We define a scaled time,

$$\tau \equiv \sqrt{\frac{g}{L}} t \quad (\text{S7})$$

so that the equation of motion reduces further to

$$\frac{d^2\theta}{d\tau^2} + \sin \theta = 0 \quad (\text{S8})$$

Once the solution  $\theta(\tau)$  is found, it can be converted back to a function the physical time  $\theta(\sqrt{\frac{g}{L}} t)$ . If the pendulum is at rest initially with an amplitude  $\theta_0$ , the solution of Eq. (S8) is typically written in the literature as

$$\theta(\tau) = 2 \arcsin[k \operatorname{sn}(\tau + K, k)] \quad (\text{S9})$$

see [DLMF, 22.19.E2](#). Here,  $k = \sin \frac{\theta_0}{2}$ .  $\operatorname{sn}(z, k)$  is one of the Jacobi elliptic functions; and  $K$  is the complete elliptical integral of the first kind, which in this context is a quarter of the period of the pendulum. However, the time dependent can be shifted from the quarter period  $K$  back to zero by using the relation

$$\operatorname{sn}(z + K, k) = \operatorname{cd}(z, k) \quad (\text{S10})$$

see [DLMF, 22.4.T3](#).  $\operatorname{cd}(z, k)$  is another Jacobi elliptic function. Therefore, the solution takes the form

$$\theta(\tau) = 2 \arcsin[k \operatorname{cd}(\tau, k)] \quad (\text{S11})$$

To avoid the  $\arcsin[\dots]$  dependent above and steering toward a simpler Fourier form, the following integral property is used.

$$\int \operatorname{sd}(x, k) dx = -\frac{1}{kk'} \arcsin[k \operatorname{cd}(x, k)] \quad (\text{S12})$$

see [DLMF, 22.14.E5](#). Note that the minus sign is taken out of  $\arcsin[\dots]$  function, as compared to the reference.  $\operatorname{sd}(z, k)$  is one of the Jacobi elliptic function. Therefore, the solution can now be written as

$$\theta(\tau) = -2kk' \int \operatorname{sd}(\tau, k) d\tau \quad (\text{S13})$$

A fourier expansion of  $\operatorname{sd}(z, k)$  is also available. It reads

$$\operatorname{sd}(z, k) = \frac{2\pi}{Kkk'} \sum_{n=0}^{\infty} \frac{(-1)^n q^{n+\frac{1}{2}} \sin((2n+1)\zeta)}{1 + q^{2n+1}} \quad (\text{S14})$$

see [DLMF, 22.11.E5](#). The auxillary variables defined in the reference are:

$k' = \sqrt{1 - k^2}$ ,  $q = e^{-\pi K(k')/K(k)}$ ,  $\zeta = \frac{\pi z}{2K(k)}$ . Before going any further, it is convenient to adjust the form of the summation index  $n$ . Note that  $(2n + 1)$  is always an odd integer, so we define an odd integer  $m = (2n + 1)$ . The above Fourier expansion becomes

$$\text{sd}(\tau, k) = \frac{2\pi}{Kk k'} \sum_{m \text{ odd}} \frac{(-1)^{\frac{m-1}{2}} q^{\frac{m}{2}} \sin(\frac{m\pi}{2K}\tau)}{1 + q^m} = \frac{2\pi}{Kk k'} \sum_{m \text{ odd}} \frac{(-1)^{\frac{m-1}{2}} \sin(\frac{m\pi}{2K}\tau)}{2 \cosh(\kappa m\pi/2)} \quad (\text{S15})$$

Here, we define  $\kappa \equiv \frac{K(\sqrt{1-k^2})}{K(k)}$ . Substutute  $\text{sd}(\tau, k)$  above into the integral in Eq. (S13). The solution becomes

$$\theta(\tau) = -\frac{2\pi}{K} \sum_{m \text{ odd}} \frac{(-1)^{\frac{m-1}{2}}}{\cosh(\kappa m\pi/2)} \int \sin(\frac{m\pi}{2K}\tau) d\tau \quad (\text{S16})$$

Here, the integration is pushed through the summation to meet the time dependent  $\sin(\frac{m\pi}{2K}\tau)$ . The integration can easily be performed, yielding

$$\theta(\tau) = \sum_{m \text{ odd}} \frac{(-1)^{\frac{m-1}{2}}}{m} \frac{4}{\cosh(\kappa m\pi/2)} \cos(\frac{m\pi}{2K}\tau) \quad (\text{S17})$$

However,  $4K$  can be interpreted as the period in the scaled time  $\tau$ . Therefore,

$$\cos(\frac{m\pi}{2K}\tau) = \cos(\frac{2m\pi}{4K}\tau) \quad (\text{S18})$$

Notice the ratio of the scaled time  $\tau$  to its period  $4K$ . Upon converting from the scaled time to the physical time  $\tau \rightarrow \sqrt{\frac{g}{L}}t$ , so is the period  $4K \rightarrow \sqrt{\frac{g}{L}}T$ . Hence, the factor  $\sqrt{\frac{g}{L}}$  is eliminated inside the cosine fuctions.

Renaming the index  $m \rightarrow n$ , the series becomes.

$$\theta(t) = \sum_{n \text{ odd}} a_n \cos(\frac{2n\pi}{T}t) \quad (\text{S19})$$

where the Fourier coefficients (only for n odd) are

$$a_n = \frac{(-1)^{\frac{n-1}{2}}}{n} \frac{4}{\cosh(\kappa n\pi/2)}, \quad \kappa \equiv \frac{K(\sqrt{1-k^2})}{K(k)} \quad (\text{S20})$$

But the series in Eq.(S19) when the pendulum starts at rest at the initial angle  $\theta_0$ . Shifting the by a quarter of the period causes the pendulum to start at the bottom, with initial angular speed  $\omega_m$  to jump start the motion.

$$\theta(t) = \sum_{n \text{ odd}} a_n \cos(\frac{2n\pi}{T}t - \frac{n\pi}{2}) \quad (\text{S21})$$

Use a simple trigonometry identity  $\cos(A - B) = \cos A \cos B + \sin A \sin B$  and the fact that  $n$  is always an odd number, we have

$$\theta(t) = \sum_{n \text{ odd}} a_n (-1)^{\frac{n-1}{2}} \sin(\frac{2n\pi}{T}t) \quad (\text{S22})$$

The alternating  $\pm 1$  sign can be absorbed into  $a_n$ , leading to an even simpler form

$$\theta(t) = \sum_{n \text{ odd}} a_n \sin(\frac{2n\pi}{T}t + n\delta) \quad (\text{S23})$$

$$a_n = \frac{4}{n \cosh(\kappa n\pi/2)}, \quad \kappa \equiv \frac{K(\sqrt{1-k^2})}{K(k)} \quad (\text{S24})$$

## the Phase Constant

The phase constant  $\delta$  for the swinging motion can be computed by finding a root of

$$f(\delta) = 0 = \theta_0 - \sum_{n \text{ odd}} a_n \sin(n\delta) \quad (\text{S25})$$

For Newton root finding method, an initial guess of  $\delta_0$  need to be given. The successive values of  $\delta_n$  can be updated using

$$\delta_{n+1} = \delta_n - \frac{f(\delta_n)}{f'(\delta_n)} \quad (\text{S26})$$

The iterations stop when the  $\delta_n$  converges. The initial guess  $\delta_0$  can be determined from using only the first term in the summation, namely.

$$0 = \theta_0 - a_1 \sin(\delta_0) \quad (\text{S27})$$

Caution must be taken when solving for  $\delta_0$  because there are 2 possible solutions. The two solutions have the same value  $\theta_0$ , but opposite sign of slope, corresponding to the sign of angular velocity. Depending on the sign of  $\omega_0$ ,

$$\delta_0 = \begin{cases} \arcsin(\theta_0/a_1) & \text{if } \omega_0 > 0 \\ \pi - \arcsin(\theta_0/a_1) & \text{if } \omega_0 < 0 \end{cases} \quad (\text{S25})$$

In the python example below, the iterations in Eq. (S26) continue until  $\delta_{n+1}$  differs from  $\delta_n$  smaller than  $10^{-8}$ . The converged value of  $\delta$  is then used to plot  $\theta(t)$ .

```
In [5]: #
# This python shows how to compute the phase constant
# delta for all 3 classes of motion.
#

import numpy as np
import matplotlib.pyplot as plt

# compute phase shift for swinging motion delta using newton method
def phase_shift(theta0, omega0, cutoff):

    # compute omegaM
    omegaM = np.sqrt(omega0**2 - 2*g/L*np.cos(theta0) + 2*g/L)

    # swinging motion
    if omegaM < omegac:

        # compute coefficient an
        k = np.sqrt(L/g)*omegaM/2
        kappa = K(np.sqrt(1-k**2))/K(k)

        N = 20
        a = np.zeros(N)
        for j in range(1,N,2):
            a[j] = 4/j/np.cosh(kappa*j*np.pi/2)

        def f(delta):
            s = 0
            for j in range(1,N,2): s = s + a[j]*np.sin(j*delta)
            return theta0 - s

        def fp(delta):
            s = 0
            for j in range(1,N,2): s = s + j*a[j]*np.cos(j*delta)
            return -s

        # initial guess
        if theta0 == 0.0: return 0.0
        if omega0 == 0.0:
            if theta0 > 0: return +np.pi/2
            else: return -np.pi/2

        delta = np.arcsin(theta0/a[1])
        if omega0 < 0: delta = np.pi - delta

        # update
        while True:
            step = - f(delta)/fp(delta)
            delta = delta + step
```

```

        if np.abs(step) < cutoff: break

# stopping motion
elif omegaM == omegac:
    k = np.sin(theta0/2)
    delta = 1/2*np.log((1+k)/(1-k))

# spinning motion
else:

    # compute coefficients
    N = 20
    b = np.zeros(N)
    k = np.sqrt(L/g)*omegaM/2
    kappa = K(np.sqrt(1-1/k**2))/K(1/k)
    for n in range(1,N):
        b[n] = 2/n/np.cosh(n*np.pi*kappa)

    def f(delta):
        s = 0
        for j in range(1,N,1): s = s + b[j]*np.sin(j*delta)
        return theta0 - delta - s

    def fp(delta):
        s = 0
        for j in range(1,N,1): s = s + j*b[j]*np.cos(j*delta)
        return -1-s

    # initial guess
    if theta0 == 0.0: return 0.0
    delta = theta0/(1+b[1])

    # update
    while True:
        step = - f(delta)/fp(delta)
        delta = delta + step
        if np.abs(step) < cutoff: break

    return delta

Tmax = 4
t = np.arange(0,Tmax,0.01)

# case 1) swinging starting at theta0 = pi/2
theta0 = np.pi/2
omega0 = np.sqrt(omegac**2 + 2*g/L*np.cos(theta0) - 2*g/L) - 0.001
omegaM = np.sqrt(omega0**2 - 2*g/L*np.cos(theta0) + 2*g/L)
delta = phase_shift(theta0, omega0, 1e-8)
#theta_swinging = theta_CKS(omegaM, t, delta)
theta_swinging = theta_CKS(omegaM, t, -np.pi)

# case 2) stopping starting at theta0 = pi/2
theta0 = np.pi/2
omega0 = np.sqrt(omegac**2 + 2*g/L*np.cos(theta0) - 2*g/L)
omegaM = np.sqrt(omega0**2 - 2*g/L*np.cos(theta0) + 2*g/L)
delta = phase_shift(theta0, omega0, 1e-8)
theta_stopping = theta_CKS(omegaM, t, delta)

# case 3) spinning starting at theta0 = pi/2
theta0 = np.pi/2
omega0 = np.sqrt(omegac**2 + 2*g/L*np.cos(theta0) - 2*g/L) + 0.001
omegaM = np.sqrt(omega0**2 - 2*g/L*np.cos(theta0) + 2*g/L)
delta = phase_shift(theta0, omega0, 1e-8)
theta_spinning = theta_CKS(omegaM, t, delta)

plt.plot(t, theta_swinging, '--', label='Swinging:  $\theta_0 = \pi/2$ ')
plt.plot(t, theta_stopping, '-.', label='Stopping:  $\theta_0 = \pi/2$ ')
plt.plot(t, theta_spinning, '-', label='Spinning:  $\theta_0 = \pi/2$ ')
plt.ylim(-np.pi,4*np.pi)
plt.xlim(0,Tmax)
plt.yticks([-np.pi,0,np.pi,2*np.pi,3*np.pi,4*np.pi],
           ['$-\pi$', '0', '$\pi$', '$2\pi$', '$3\pi$', '$4\pi$'])
plt.xticks([0,1,2,3,4])
plt.grid()
plt.legend()
plt.xlabel('Time [seconds]')
plt.ylabel('Angular Displacement')

```

```
#plt.savefig('fig4.pdf')
plt.show()
```

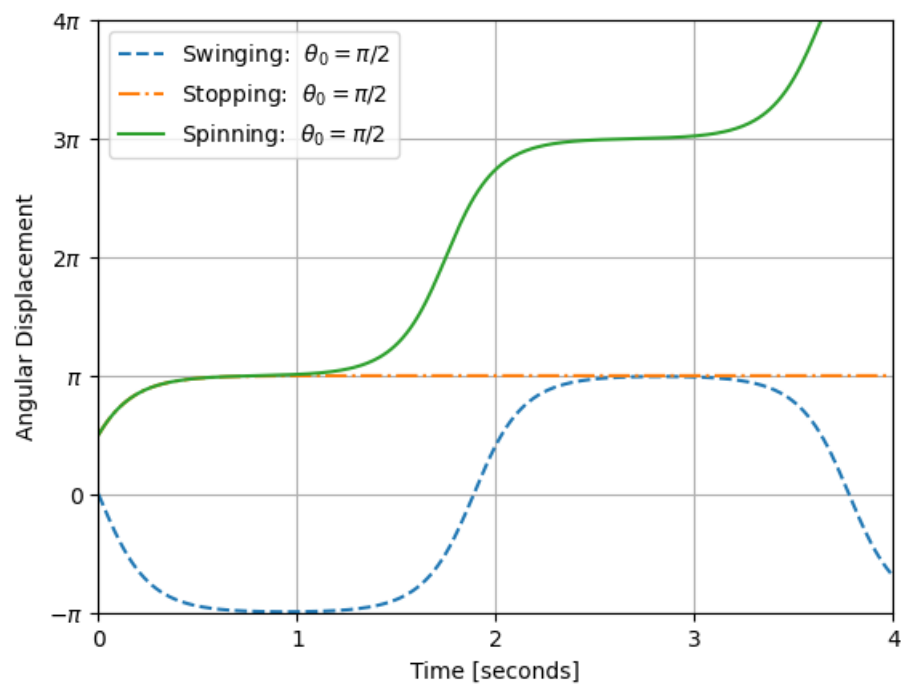

## References

Ganley, W. P. (1985). Simple pendulum approximation. *American Journal of Physics*, 53(1), 73–76.  
<https://doi.org/10.1119/1.13970>

Lima, F. M. S. (2008). Simple 'log formulae' for pendulum motion valid for any amplitude. *European Journal of Physics*, 29(5), 1091–1098. <https://doi.org/10.1088/0143-0807/29/5/021>

[DLMF] NIST Digital Library of Mathematical Functions. <https://dlmf.nist.gov/>, Release 1.2.4 of 2025-03-15. F. W. J. Olver, A. B. Olde Daalhuis, D. W. Lozier, B. I. Schneider, R. F. Boisvert, C. W. Clark, B. R. Miller, B. V. Saunders, H. S. Cohl, and M. A. McClain, eds.

In [ ]:
